# Supplementary material for: High-dimensional Bayesian Model for Disease-Specific Gene Detection in Spatial Transcriptomics
Source: arXiv:2409.02397 source file (2024-09-04)
Supplement: Supplementary file 1 [file Appendix.tex]

\documentclass{article}
\begin{document}

\input{table/Table 3 eta=0.1}

\end{document}
